# Supplementary material for: What is wrong with you?: Leveraging User Sentiment for Automatic Dialog Evaluation
Source: arXiv:2203.13927 source file (2022-03-25)
Supplement: Supplementary file 1 [file appendix2021.tex]

% This must be in the first 5 lines to tell arXiv to use pdfLaTeX, which is strongly recommended.
\pdfoutput=1
% In particular, the hyperref package requires pdfLaTeX in order to break URLs across lines.

\documentclass[11pt]{article}

% Remove the "review" option to generate the final version.
\usepackage[review]{emnlp2021}

% Standard package includes
\usepackage{times}
\usepackage{latexsym}

% For proper rendering and hyphenation of words containing Latin characters (including in bib files)
\usepackage[T1]{fontenc}
% For Vietnamese characters
% \usepackage[T5]{fontenc}
% See https://www.latex-project.org/help/documentation/encguide.pdf for other character sets

% This assumes your files are encoded as UTF8
\usepackage[utf8]{inputenc}

% This is not strictly necessary, and may be commented out,
% but it will improve the layout of the manuscript,
% and will typically save some space.
\usepackage{microtype}

\usepackage{graphicx}
\usepackage{arydshln}
\usepackage{multirow}

% If the title and author information does not fit in the area allocated, uncomment the following
%
%\setlength\titlebox{<dim>}
%
% and set <dim> to something 5cm or larger.

\begin{document}
\appendix

\section{Appendices}
\label{sec:appendix}

%\section{Supplemental Material}
%\label{sec:supplemental}

\end{document}
